# Supplementary material for: DexLego: Reassembleable Bytecode Extraction for Aiding Static Analysis
Source: arXiv:1803.02471 source file (2018-04-15)
Supplement: Supplementary file 1 [file appendix.tex]

%\newpage
%\section{Network Protocol} 
%\label{sec:protocol}
